# Supplementary material for: Logit-Aware MIMO AirComp for Distributed Mixture-of-Experts LLM Inference over Wireless Edge Networks
Source: arXiv:2610.03741 source file (2026-09-22)
Supplement: Supplementary file 1 [file appendix_proofs.tex]

\appendices
\section{Proofs}

\subsection{Proof of Lemma~\ref{lem:scalar-sensitivity-reduction}}
\label{app:proof-scalar-sensitivity}

\begin{proof}
Under the first-order approximation,
\begin{equation}
    \widehat{\bo}_t-\bo_t
    \approx
    \bJ_{\ell,t}\bdelta_t^{(\ell)} .
\end{equation}
Therefore,
\begin{align}
    \E\left[
    \left\lVert
    \widehat{\bo}_t-\bo_t
    \right\rVert_2^2
    \right]
    &\approx
    \E\left[
    \bdelta_t^{(\ell)T}
    \bQ_{\ell,t}
    \bdelta_t^{(\ell)}
    \right] \nonumber\\
    &=
    \sum_{b\in\cB_{t,\ell}}
    \Tr\left(
    \mathbf G_b^T
    \bQ_{\ell,t}
    \mathbf G_b
    \E\left[
    \mathbf r_b\mathbf r_b^T
    \right]
    \right),
    \label{eq:proof-scalar-step1}
\end{align}
where the cross-resource terms vanish because the resource errors are
mutually uncorrelated. Using \eqref{eq:isotropic-resource-error}, we have
\begin{align}
    \E\left[
    \left\lVert
    \widehat{\bo}_t-\bo_t
    \right\rVert_2^2
    \right]
    &\approx
    \sum_{b\in\cB_{t,\ell}}
    \frac{\epsilon_b}{q_b}
    \Tr\left(
    \mathbf G_b^T
    \bQ_{\ell,t}
    \mathbf G_b
    \right) \nonumber\\
    &=
    \sum_{b\in\cB_{t,\ell}}
    \omega_b\epsilon_b .
\end{align}
This completes the proof.
\end{proof}

\subsection{Proof of Theorem~\ref{thm:sensitivity-bound}}
\label{app:proof-sensitivity-bound}
\begin{proof}
Taylor's theorem gives
\begin{equation}
    \widehat{\bo}_t-\bo_t
    =
    \bJ_{\ell,t}\bdelta_t^{(\ell)}
    +
    \mathbf r_{\ell,t},
\end{equation}
where the local Lipschitz continuity of the Jacobian implies
\begin{equation}
    \|\mathbf r_{\ell,t}\|_2
    \le
    \frac{L_{\ell,t}}{2}
    \|\bdelta_t^{(\ell)}\|_2^2.
\end{equation}
Using
\begin{equation}
    \|\mathbf a+\mathbf b\|_2^2
    \le
    (1+\rho)\|\mathbf a\|_2^2
    +
    (1+\rho^{-1})\|\mathbf b\|_2^2
\end{equation}
with $\mathbf a=\bJ_{\ell,t}\bdelta_t^{(\ell)}$ and $\mathbf b=\mathbf r_{\ell,t}$, and then taking expectation, gives \eqref{eq:sensitivity-upper-bound}. Substituting \eqref{eq:weighted-mse-reduction} gives
\eqref{eq:sensitivity-weighted-upper-bound}.
\end{proof}

\subsection{Proof of Corollary~\ref{cor:token-preservation}}
\label{app:proof-token-preservation}
\begin{proof}
If every logit moves by less than $\Gamma_t/2$ in absolute value, the clean winning logit can decrease by at most $\Gamma_t/2$, and every competing logit can increase by at most $\Gamma_t/2$. Therefore, the clean winner remains above every competitor. The probability bound follows from
\begin{equation}
    \|\widehat{\bo}_t-\bo_t\|_\infty
    \le
    \|\widehat{\bo}_t-\bo_t\|_2
\end{equation}
and Markov's inequality.
\end{proof}

\subsection{Proof of Lemma~\ref{lem:mse-decomposition}}
\label{app:proof-mse-decomposition}
\begin{proof}
Using \eqref{eq:received-signal}--\eqref{eq:linear-detector}, the AirComp error on resource $b$ is
\begin{equation}
    \widehat{\bs}_{\Sigma,b}
    -
    \bs_{\Sigma,b}
    =
    \sum_{m\in\cM_t^{(\ell)}}
    \left(
    \bA_b^H
    \bH_{m,b}
    \bF_{m,b}
    -
    \bI_r
    \right)
    \bs_{m,b}
    +
    \bA_b^H\bw_b .
\end{equation}
Taking $\E[\|\widehat{\bs}_{\Sigma,b}-\bs_{\Sigma,b}\|_2^2]$, the cross terms among different BSs vanish because the sources are zero mean and mutually independent. The cross terms between source vectors and noise vanish by independence. The noise term is
\begin{equation}
    \E\!\left[
    \|\bA_b^H\bw_b\|_2^2
    \right]
    =
    \sigma_b^2
    \Tr(\bA_b^H\bA_b).
\end{equation}
This proves \eqref{eq:mse-decomposition}.
\end{proof}

\subsection{Proof of Proposition~\ref{prop:block-convexity}}
\label{app:proof-block-convexity}
\begin{proof}
The combiner objective has the quadratic form in \eqref{eq:combiner-quadratic}. Since $\mathbf R_{y,b}\succ\bzero$, its Hessian is positive definite in the real-equivalent representation of $\bA_b$, so the minimizer is unique. For the precoders, each term in \eqref{eq:precoder-convex-objective} is a squared norm of an affine function of $\bF_{m,b}$, weighted by $\omega_b\ge0$. The power constraints are sublevel sets of convex quadratic functions because $\bR_{m,b}\succeq\bzero$. Hence the fixed-combiner subproblem is convex, and its KKT conditions are sufficient for global optimality.
\end{proof}

\subsection{Proof of Proposition~\ref{prop:combiner}}
\label{app:proof-combiner}
\begin{proof}
The estimate $\widehat{\bs}_{\Sigma,b}=\bA_b^H\by_b$ is linear in $\by_b$. For fixed precoders, minimizing
\begin{equation}
    \E\!\left[
    \|\bA_b^H\by_b-\bs_{\Sigma,b}\|_2^2
    \right]
\end{equation}
over $\bA_b$ is a linear MMSE estimation problem. The corresponding normal equation is
\begin{equation}
    \mathbf R_{y,b}\bA_b
    =
    \mathbf R_{ys,b}.
\end{equation}
Substituting \eqref{eq:received-signal} and using Assumption~\ref{ass:source} yields \eqref{eq:Ry} and \eqref{eq:Rys}. Since $\sigma_b^2>0$, $\mathbf R_{y,b}$ is positive definite.
\end{proof}

\subsection{Proof of Proposition~\ref{prop:precoder}}
\label{app:proof-precoder}
\begin{proof}
For fixed $\{\bA_b\}$, the terms depending on $\bF_{m,b}$ are
\begin{align}
    \sum_{b\in\cB_m}
    \omega_b
    \Tr\!\big(&
    (\bA_b^H\bH_{m,b}\bF_{m,b}-\bI_r)
    \bR_{m,b}
    \nonumber\\
    &\times
    (\bA_b^H\bH_{m,b}\bF_{m,b}-\bI_r)^H
    \big)
\end{align}
plus the total-power and peak-power constraint terms. The Lagrangian terms involving $\bF_{m,b}$ include
\begin{equation}
    \lambda_m
    \Tr(\bF_{m,b}\bR_{m,b}\bF_{m,b}^H)
    +
    \nu_{m,b}
    \Tr(\bF_{m,b}\bR_{m,b}\bF_{m,b}^H).
\end{equation}
Taking the Wirtinger derivative with respect to $\bF_{m,b}^\ast$ gives
\begin{align}
    &\omega_b
    \bH_{m,b}^H
    \bA_b
    \left(
    \bA_b^H
    \bH_{m,b}
    \bF_{m,b}
    -
    \bI_r
    \right)
    \bR_{m,b}
    \nonumber\\
    &\quad+
    (\lambda_m+\nu_{m,b})
    \bF_{m,b}
    \bR_{m,b}
    =
    \bzero.
    \label{eq:precoder-kkt-stationarity}
\end{align}
On the support of $\bR_{m,b}$, this yields
\begin{equation}
    \omega_b \bM_{m,b}\bF_{m,b}
    =
    \omega_b \bH_{m,b}^H\bA_b .
\end{equation}
Dividing by $\omega_b>0$ gives \eqref{eq:optimal-precoder-weighted}.
\end{proof}

\subsection{Proof of Proposition~\ref{prop:monotonicity}}
\label{app:proof-monotonicity}
\begin{proof}
For fixed precoders, \eqref{eq:optimal-combiner} minimizes each resource MSE over the linear combiner. For fixed combiners, the precoder subproblem is convex in each BS's precoder variables under the quadratic power constraints, and its KKT solution minimizes that block update. Hence no alternating step increases the objective. The objective is lower bounded by zero, so the values converge. Standard block-coordinate descent arguments imply block-stationarity of accumulation points.
\end{proof}
